# Supplementary material for: Navigating protein landscapes with a machine-learned transferable coarse-grained model
Source: arXiv:2310.18278 ancillary file (2023-10-27)
Supplement: Supplementary file 1 [file SI.pdf]

# Supplementary Information

## S1 Data Preparation

### S1.1 Octapeptides

In order to parametrize the transferable prior model for the delta learning scheme, a diverse set of octapeptide sequences were simulated using molecular dynamics (MD) to create a fitting dataset for the interactions described in Section S2. A set of candidate sequences was picked from the PISCES database [1] using default query parameters and was cut into 3,326,176 octapeptide subsequences. Each subsequence was featurized into a 6-dimensional vector containing the following physicochemical properties from Table 3 in [2]: RF (chromatographic relative-to-front) rank, bulkiness, pK1, isoelectric point (pI), hydrophobicity, and polarity. Principal component analysis (PCA) was then used to obtain a reduced-dimension representation of these features across all peptides by projecting onto the first two principal components. K-means clustering was then performed in this reduced space with 2000 cluster centers. Random subsequences were sampled from the cluster centers until 1100 unique subsequences were obtained.

All atomistic peptide simulations used the AMBER ff-99SB-ILDN force field [3] and the TIP3P water model [4]. For each of the 1100 sequences, an octapeptide structure was generated using PyMol [5]. These structures were then solvated and equilibrated using Langevin dynamics in ACEMD [6]. All heavy-hydrogen bonds were constrained, the hydrogen masses were increased by a factor of 4, PME was utilized with a 1.0 nm grid spacing, for nonbonded interactions a cutoff at 0.9nm and a switching distance of 0.75 nm were employed, the friction constant was set to 0.1 $ps^{-1}$, and a timestep of 4 fs was used. Systems were neutralized and simulated at a concentration of 0.1M NaCl. Production simulations at 300K were run for each peptide, in which the adaptive sampling strategy described in [7] was used to generate around 100 all-atom trajectories, each about 10 ns long for a total of 1 $\mu$s simulation time for each peptide. The entire completed dataset consisted of 1.1 ms of all-atom simulation coordinates and forces.

Two peptides, DYGCSIHP and SLEAGGRG, were selected for further, longer simulation in order to prepare reference free energy surfaces (FESs) to test the extrapolation of the transferable CGSchNet. For each of these two peptides, an initial configuration was chosen randomly from the original octapeptide dataset described above, and a single, long, all-atom MD simulation was performed with the same settings in OpenMM for a total of 3.5 microseconds, saving every 2 ps.

In order to ensure a complete convergence of the simulation an MSM was evaluated for the two molecules. Considering sin and cos of the $\phi$ and $\psi$ dihedral angles, together

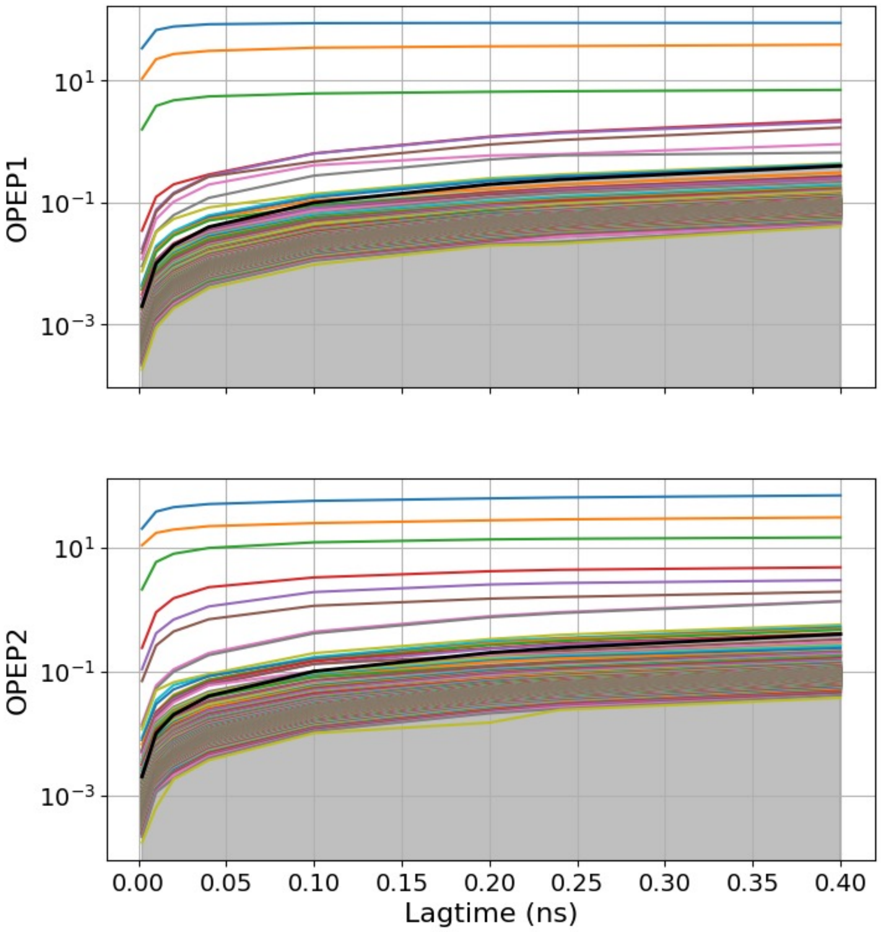


**Fig. S1**: MSM implied timescales for the two chosen reference peptides. The units of the y-axis are in ns. OPEP1 refers to DYGCSIHP and OPEP2 refers to SLEAGGRG.

with the distance between all $C_{alpha}$ atoms as features, a TICA model was built taking a lag-time of 1000 frames (2 ns). This model was also used to project the CG simulation results. A k-means clustering with 500 cluster centers was then performed for the estimation of a maximum likelihood MSM using a lagtime of 20 frames (0.04 ns). This later was used to reweight the trajectory. Fig. S1 shows the converged of the MSM implied timescales for both systems.

## S1.2 Dimers

1245 systems of capped mono/dipeptide dimer pairs for a variety of sequences were solvated and prepared using OpenMM [8]. Umbrella sampling simulations were carried

out with the center of mass (COM) distance between the molecules as a reaction coordinate, which varied on a linear grid between 3 and 30 Å using a force constant of 500 kJ/mol/nm$^2$. The same force field, temperature, and simulation settings were used as described in Section S1.1, though the integration timestep was set to 2 fs and no hydrogen mass re-partitioning was in effect. At each window, systems were equilibrated using NPT for 50 ps with a high friction constant 100 ps$^{-1}$, followed by production simulation for 1 ns. Protein coordinates and forces were saved from production runs every 1 ps. Configurations were used without reweighting for force-matching.

## S1.3 CATH Domains

A set of candidate 14942 non-redundant structural domains was selected from the CATH database [9]. From this set, domains were further excluded if: 1) they contained non-contiguous structures/sequences, 2) they had less than 50 residues, 3) they had more than 75 residues, 4) they had a relative shape anisotropy of $> 0.04$, or 5) they had a combined helix and sheet fraction (as defined by coarse DSSP [10] using MDTraj [11]) of less than 50 percent. Applying these exclusions resulted in a compact set of 95 non-redundant domains. From this set, a final set of 50 domains, with a nearly equal fraction of helix to beta-sheet secondary structure, was formed. These domains and their sequence lengths are enumerated in Table S1. A tiled ribbon representation of all 50 chosen CATH domains is shown in Fig. S2.

For each sequestered CATH domain in the final set, structures and topologies were processed from MD simulations using OpenMM and tools from GROMACS [12]. Each domain was solvated and equilibrated using Gromacs with the same force field and simulation parameters used in Section S1.1, except that the thermostat friction is set to 1 ps$^{-1}$. After this, four 0.5-$\mu$s production all-atom simulations using Langevin dynamics were run for each domain in OpenMM, resulting in 2 $\mu$s of simulation for each domain and 100 $\mu$s of simulation coordinates and forces across all final CATH domains. Coordinates and forces of protein atoms were stored at a 20 ps interval.

## S1.4 Training and Validation Set

Training and validation sets were constructed exclusively from the dimer and folded CATH simulations; the octapetides were only used as part of the prior model parametrization (see Section S2). To construct the training and validation sets for the network, dataset splits were made on a *molecular* basis. That is, for each subdataset (dimer or CATH), the molecule identities of that subdataset were further partitioned according to a random 80/20 % train/validation split. In the end, the training/validation set each consists of a selection of dimer molecules and of CATH molecules. Furthermore, 6 purely helical CATH domains were discarded from the final CATH training set to better balance the ratio of helix to sheet structures. In this way, the validation loss assessed how well the model was learning to predict CG forces on sets of molecules (sequences and structures) that were never seen by the network during training.

| Domain ID | Length | Domain ID | Length | Domain ID | Length |
|---|---|---|---|---|---|
| 1b43A02 | 61 | 1z1vA00 | 70 | 3a5zD02 | 64 |
| 1bl0A02 | 60 | 2au3A04 | 55 | 3e6zX01 | 75 |
| 1c75A00 | 71 | 2bh1X00 | 68 | 3ethA03 | 62 |
| 1d3yA01 | 71 | 2cg5B00 | 71 | 3g7lA00 | 55 |
| 1iz6A02 | 64 | 2ckkA01 | 53 | 3goxA01 | 51 |
| 1ldjA06 | 68 | 2dkzA01 | 61 | 3luyA02 | 74 |
| 1mpgA03 | 52 | 2dl0A01 | 59 | 3ossC00 | 65 |
| 1neqA00 | 74 | 2e8oA01 | 62 | 3tj8A02 | 74 |
| 1o82A00 | 70 | 2f48A03 | 75 | 3udcA02 | 50 |
| 1on2A01 | 72 | 2ga1A02 | 70 | 3vseA01 | 69 |
| 1r3fA02 | 65 | 2hbpA00 | 66 | 4a53A01 | 62 |
| 1s6lA01 | 52 | 2heoA00 | 59 | 4hwiB01 | 71 |
| 1skyB01 | 70 | 2htjA01 | 60 | 4jriB00 | 64 |
| 1sxjE02 | 64 | 2hyvA01 | 73 | 4kdiD00 | 75 |
| 1w0tA00 | 52 | 2nttA02 | 70 | 4npsA02 | 58 |
| 1wfxA01 | 71 | 2v0cA03 | 57 | 4o96A01 | 73 |
| 1xovA03 | 72 | 2wg5F02 | 58 | | |

**Table S1**: Chosen set of 50 CATH domains with their respective sequence lengths.

## S1.5 Fast Folders

To generate the reference data used to validate the CG model, we simulated several proteins found in or similar to the fast folder suite studied by Lindorff-Larsen et al [14]. These proteins are listed in Table S4 below. Simulation parameters including the force field and the integration settings are identical to the ones described in the dimer dataset above (see Section S1.2). The sampling strategy used for each protein differed. In the case of Trpcage, BBA, and Villin, trajectories starting from different portions of phase space were used. For the remaining proteins, multiple trajectories were started from a single configuration. A summary of the aggregate simulation length and number of constituent trajectories for these proteins is given in Table S2. The trajectories for CLN025, Trpcage, BBA, and Villin were postprocessed using Markov state models (MSMs) [15].

***CLN025***
20 independent simulations were run for 5 $\mu$s with the coordinates of protein atoms saved at a 50 ps interval. All simulations were started from the same extended structure. Nonbonded cutoff was set to 1.0 nm and no switching function was used.

***Trpcage & BBA***
3525 (Trpcage) and 3295 (BBA) starting configurations were taken from a previously published study [16]. These simulation start points were selected at random from a 2D slow collective variable projection computed with TICA at a 120 ns lagtime using the pairwise distance between the carbon alpha atoms. In the case of Trpcage, the final four carbon alpha atoms were discarded as this region is highly disordered and does not correspond to large scale protein motion. In the slow collective variable space, bins were placed uniformly and 5 structures from each bin were selected and run for 500 ns with positions saved every 2 ps.

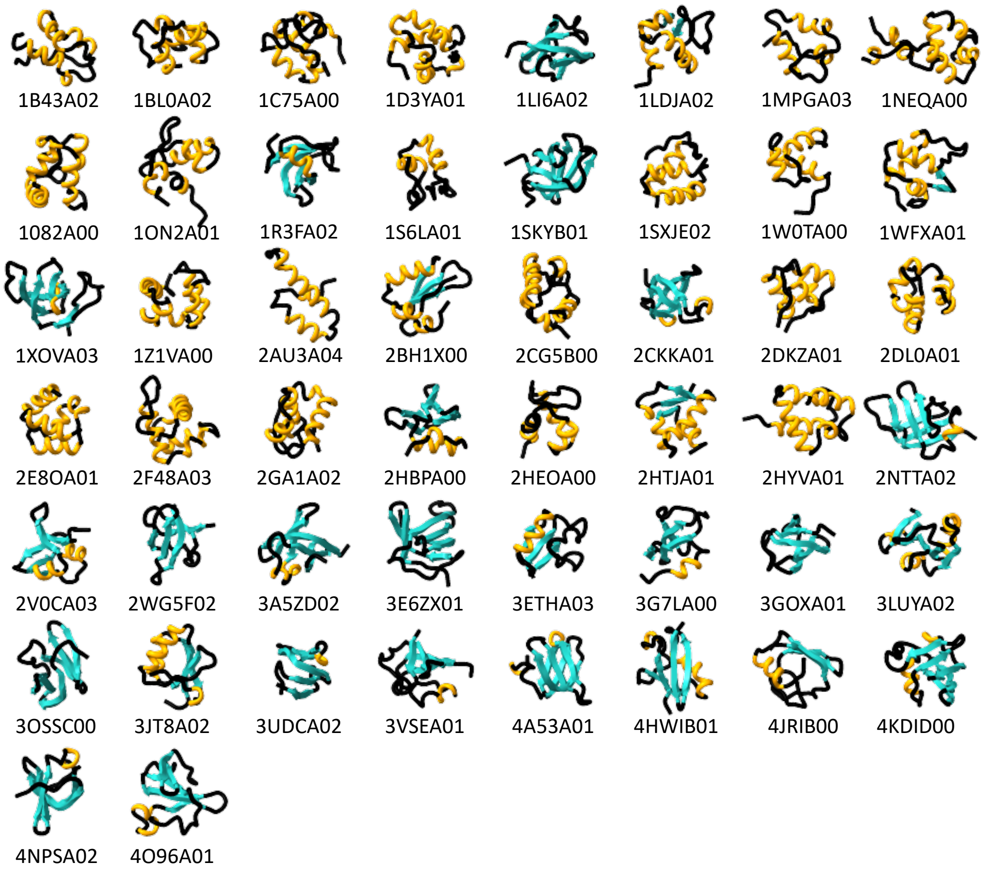


**Fig. S2**: Chosen set of 50 CATH Domains. Disordered regions are colored black, helical regions are orange, and sheet regions are blue. Figure generated using UCSF ChimeraX [13].

***Villin***

151 individual trajectories were initialized in varying parts of the Villin phase space for approximately 5 $\mu$s each. Initial simulations were started from folded and unfolded structures; after completion, simulations that explored novel parts of phase space were continued with an additional round of simulations manually spawned from their endpoints. This process was repeated two more times to generate a collection of 151 trajectories. Generated trajectories varied in exact length due to fixed walltime limits and varying hardware. 4 trajectories were removed from the analysis as they irreversibly entered misfolded states and could not be included in the MSM analysis, reflecting the fundamental difficulty in fully converging protein simulations on consumer hardware. Frames were saved every 10 ps.

***Alpha 3D & Homeodomain***

24 (Alpha 3D) and 28 (Homeodomain) MD simulations were started at the folded

structure given by the PDB. Individual simulations were approximately 5 $\mu$s. These two proteins did not exhibit unfolding nor any large-scale fluctuations during atomistic simulations. Frames were saved every 10 ps.

| Name (PDB) | # Traj. | Aggr. length ($\mu$s) | Median length ($\mu$s) |
|---|---|---|---|
| CLN025 (2RVD) | 20 | 100 | 5.0 |
| Trpcage (2JOF) | 3226 | 1613 | 0.5 |
| BBA (1FME) | 3514 | 1757 | 0.5 |
| Villin (1YRF) | 147 | 747 | 4.9 |
| Alpha 3D (2A3D) | 24 | 89 | 4.2 |
| Homeodomain (1ENH) | 28 | 78 | 3.8 |

**Table S2**: Description of atomistic MD trajectories used for analyzing select fast-folding proteins.

To obtain a converged FES from short simulation trajectories for CLN025, Trpcage, BBA, and Villin, an MSM was estimated for each ensemble of trajectories. First, TICA was performed to obtain TICs, and over this projection, the MSM analysis was performed. We discretized the trajectories using k-means clustering over the first 2 TIC coordinates and, from this discretization, a maximum-likelihood MSM was estimated. Hyperparameters for this analysis can be consulted in table S3. The lagtimes were selected after visually inspecting a plot of the implied timescales as a function of the lagtime. For Villin, as the first two processes do not converge, the lagtime was selected based on the convergence of the third process. Timescale plots are shown in Fig. S3. We note that in the case of Villin, no trajectories spontaneously unfolded and all 8 trajectories started in the unfolded state quickly refolded, supporting the conclusion that the unfolded state of Villin is not stable at these thermodynamic conditions. This phenomenon was recapitulated in the MSM reweighting process.

## S1.6 Extrapolation Target Sequence similarity

We define the sequence similarity, $o$, for a target sequence $S_T$ and a reference sequence $S_R$ as $o = (\text{Num. Matching Residues})/|\text{Align}(S_T, S_R)|$ where "Align" is a lexicographic alignment function and $|\cdot|$ represents the length of an alignment. For alignments, we use Biopython's `pairwise2.align.localxs` function [18], with gap

| Protein | TICA input features | # clusters | Lagtime (ns) |
|---|---|---|---|
| CLN025 | Pairwise CA distances | 500 | 5 |
| Trpcage | Pairwise CA distances of all but the first residue | 500 | 5 |
| BBA | Sine and cosine of CA dihedral angles | 350 | 5 |
| Villin | Pairwise CA distances | 250 | 250 |

**Table S3**: MSMs hyperparameters. The MSMs were estimated using the Deeptime library [17].

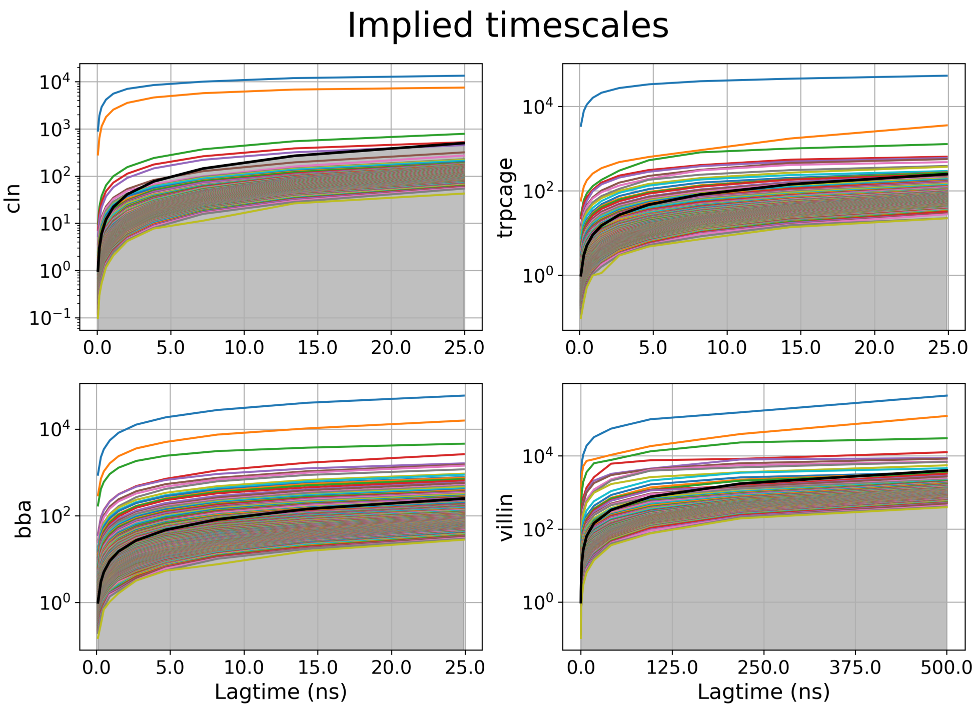


**Fig. S3**: MSM implied timescales as functions of lagtime for the proteins. Y-axis uses nanosecond unit with log-scale.

open and extend penalties both set to $-1$. Thus, the sequence similarity in this case is just the number of matching amino acids normalized by the total length of the sequence alignment. Table S4 shows the maximum sequence similarity (rounded to the nearest whole percent) with the CATH domains for each extrapolation target used in this work. All 50 CATH domains were considered in this analysis.

# S2 Prior Model

Table S5 enumerates the features, interaction types, and specificity of priors that together constitute the prior model. All terms in the prior model are fit and fixed *before* the neural network begins training. Parametrization of each prior term (aside from the repulsions) was achieved through SciPy [19] curve fitting. Harmonic interactions have the following form:

$$V(x) = V_0 + k(x - x_0)^2 \tag{1}$$

where $x$ can either be a pairwise distance or a triplet angle, $V_0$ is constant offset, $k$ is a stiffness constant, and $x_0$ is an equilibrium distance/angle. All dihedral priors (including the two improper dihedrals, $\Gamma_{1/2}$) are parametrized to the following truncated Fourier series:

| Target | Target Sequence Length | Sequence Overlap (%) |
|---|---|---|
| DYGCSIHP | 8 | 38 |
| SLEAGGRG | 8 | 50 |
| CLN025 (2RVD) | 10 | 40 |
| Trpcage (2JOF) | 20 | 35 |
| BBA (1FME) | 28 | 31 |
| Villin (1YRF) | 35 | 30 |
| Homeodomain (1ENH) | 54 | 22 |
| SH3 (2NUZ) | 55 | 25 |
| CI2 (2CI2) | 65 | 26 |
| PaaA2 (3ZBE) | 71 | 18 |
| Alpha 3D (2A3D) | 73 | 25 |
| S6 (1RIS) | 97 | 22 |

**Table S4**: Maximum sequence similarities of extrapolation targets to CATH domains.

$$V(\theta) = V_0 + \sum_{n=1}^{n_{\text{deg}}} k_{1,n} \sin(n\theta) + k_{2,n} \cos(n\theta) \tag{2}$$

where $V_0$ is again a constant offset, $n_{\text{deg}}$ determines the maximum frequency term, and $k1/2$ are strength coefficients for each *sin* and *cos* term respectively. For phi dihedrals, all amino acids were constrained to $n_{deg} = 3$, except for PRO, which was constrained to $n_{deg} = 1$. For psi dihedrals, all amino acids were constrained to $n_{deg} = 3$. For omega dihedrals, all amino acids were constrained to $n_{deg} = 1$, except for PRO, which was fit with $n_{deg} = 2$ to allow for cis/trans isomerization. For all $\Gamma$ dihedral priors, $n_{deg} = 1$. For the prior repulsion, all atom pairs separated by 6 or more bonds contributed the following energy:

$$V(r_{ij}) = \left(\frac{\sigma_{ij}}{r_{ij}}\right)^6 \tag{3}$$

where $r_{ij}$ is the pairwise distance between atoms $i$ and $j$, and $\sigma_{ij}$ is their mutual excluded volume in 1-D. $\sigma_{ij}$ was estimated for all pair types by selecting the minimum observed pairwise simulation distance for those pair types. For C$\alpha$ and O pairs, we found it important to further increase the value to the 0.1 percentile of the observed distances in order to prevent the CG model from becoming too sticky due to otherwise poor network extrapolation.

The prior model was parametrized directly through Boltzmann inversion using the above-described octapeptide and CATH datasets (using every 100th frame to reduce memory demands). We found it necessary to fit different sets of parameters for subsets of the same type of interactions based on the general position (e.g., in the middle or on the N- or C-terminal of a peptide) and/or the chemical identity of the involved residue. Because the prior model contains no attractive interactions, it cannot stabilize compact folded states or secondary structures, such as helices or beta sheets.

| Type | CG atoms | Energy Function | Specificity |
|---|---|---|---|
| Physical Bond | $N_i^n - C_{\alpha,j}^n$ | Harmonic | N/Non/C-term |
| Physical Bond | $C_{\alpha,i}^n - C_j^n$ | Harmonic | N/Non/C-term |
| Physical Bond | $C_i^n - O_j^n$ | Harmonic | N/Non/C-term |
| Physical Bond | $C_i^n - N_j^{n+1}$ | Harmonic | N/Non/C-term |
| Physical Bond | $C_{\alpha,i}^n - C_{\beta,j}^n$ | Harmonic | N/Non/C-term/Residue |
| Physical Angle | $N_i^n - C_{\alpha,j}^n - C_k^n$ | Harmonic | N/Non/C-term |
| Physical Angle | $C_{\alpha,i}^n - C_j^n - O_k^n$ | Harmonic | N/Non/C-term |
| Physical Angle | $O_i^n - C_j^n - N_k^{n+1}$ | Harmonic | N/Non/C-term |
| Physical Angle | $N_i^n - C_{\alpha,j}^n - C_{\beta,k}^n$ | Harmonic | N/Non/C-term/Residue |
| Physical Angle | $C_{\beta,i}^n - C_{\alpha,j}^n - C_k^n$ | Harmonic | N/Non/C-term |
| Phi Dihedral | $C_i^{n-1} - N_j^n - C_{\alpha,k}^n - C_l^n$ | Fourier Series | Residue |
| Psi Dihedral | $N_i^n - C_{\alpha,j}^n - C_k^n - N_l^{n+1}$ | Fourier Series | Residue |
| Omega Dihedral | $C_{\alpha,i}^{n-1} - C_j^{n-1} - N_k^n - C_{\alpha,l}^n$ | Fourier Series | Residue |
| $\Gamma_1$ Dihedral | $N_i^n - C_{\beta,j}^n - C_k^n - C_{\alpha,l}^n$ | Fourier Series | Residue |
| $\Gamma_2$ Dihedral | $C_{\alpha,i}^n - O_j^n - N_k^{n+1} - C_l^n$ | Fourier Series | Residue |
| Repulsion | $\geq 6$ atoms apart | Inverse Power Law | CG atom type |

**Table S5**: Definition of prior energy terms. $n$ indexes the residue, while $i - l$ indexes the atom sequence defining the feature. Specificity means for each listed subset of interactions the parameters were fitted independently.

# S3 Network Model

For a molecular graph of $N$ nodes, corresponding to a CG molecule of $N$ CG atoms, a vector $\mathbf{z} \in \{0, 1, K-1\}^N$ of CG atom types are input into an initial (learnable) embedding layer that maps to embedded features $\mathbf{x}^0 \in \mathbb{R}^{N \times K}$:

$$\mathbf{x}^0 = \text{Embedding}(\mathbf{z}) \tag{4}$$

wherein $\mathbf{x}_i^0$ constitutes a vector of initial node properties for the node corresponding to the CG atom $i$. The CG atom properties are then refined through successive network *interaction blocks*, which model CG atom interactions through edge features and *continuous filters*. For a CG atom $i$, a corresponding set of edge attributes $\{E_{i1}, ..., E_{ij}, ..., E_{iJ}\}$ is generated from its $J$ CG atom neighbors contained within a finite radial cutoff, $r_{\text{cut}}$ centered on CG atom $i$. The initial edge attributes are chosen to be pairwise distances linearly expanded into a basis of $M$ univariate radial basis functions $\{f_1, ..., f_m, ...f_M\}$:

$$E_{ij} = \left[\alpha_m f_m \left(|\mathbf{r}_i - \mathbf{r}_j|\right)\right]_{m=1,\cdots,M} \tag{5}$$

where $\mathbf{r}_i \in \mathbb{R}^3$ is the Cartesian position vector of CG atom $i$ and $\{\alpha_1, ..., \alpha_M\}$ are (learnable) basis expansion coefficients. This edge information is used as input to a *filter generating network*, $\mathcal{W}(\cdot)$, whose outputs represent continuous filter values for a set of $L$ filters. The filter generating network is chosen to be a multi-layer perceptron (MLP), consisting of two linear transformations separated by an element-wise non-linear activation function $\sigma$. It is often exceedingly useful (especially for large

molecules) to apply an additional multiplicative *filter cutoff*, $\mathcal{F}(|\mathbf{r}_i - \mathbf{r}_j|)$ to the generated filters [20]. As such, the full *interaction block* refinement of the embedded CG features is defined as:

$$\mathbf{x}_i^t = \mathbf{x}_i^{t-1} + W^{t,3}\sigma\left(W^{t,2}\left(\sum_{j=1}^{J} W^{t,1}x_i^{t-1} \circ [\mathcal{F}(|\mathbf{r}_i - \mathbf{r}_j|) \circ \mathcal{W}(E_{ij})]\right)\right) \tag{6}$$

where $W^{t,1}$, $W^{t,2}$ and $W^{t,3}$ are trainable weight matrices for the linear transformations before and after convolution and activation, and embedded feature refinements are added residually to the initial node feature $\mathbf{x}_i^{t-1}$. Case $t = 1$ demonstrates how the first interaction block incorporates relative positional information of the nodes into the initial embedded features $\mathbf{x}^0$. In general, multiple interaction blocks may be assembled in series when $t \in \{1, 2, \cdots, T\}$ with $T$ representing the number of interaction blocks in the network. Analogous to deep convolutional neural networks, the continuous filter convolutions over several interaction blocks gradually incorporate information from bead pairs that are further and further apart, including those beyond the fixed cutoff radius defined for a single interaction block.

Lastly, the output of the final interaction block is fed through a small MLP that contracts down to a scalar prediction of the CG PMF:

$$U = \sum_{i=0}^{N} \mathrm{MLP}(\mathbf{x}_i^T) \tag{7}$$

from which CG forces can be extracted through a gradient operation w.r.t. to the input CG configuration coordinates and be used in a force matching loss [21].

Table S6 enumerates the SchNet neural network hyperparameters. CG atoms were integer-typed and embedded using the following strategy: integers 1-20 were used to type the $C_\beta$ atoms according to their amino acid identity (with the exception of GLY residues, in which the associated $C_\alpha$ bead was typed with the integer representing GLY), while integers 21-24 were used to type the non-$C_\beta$ atoms according to their backbone atom identity. Models were trained using data from the shuffled training set with the parameters summarized in Table S7. In every training/validation batch, the ratio of CG atoms from CATH systems to those from dimer systems was fixed to 10:1 on average (with deviations due to random size differences between sampled systems during batch construction). The final model was selected at epoch 399, after the validation loss plateaued to a near-constant value.

All training was done using PyTorch Lightning [23]. All training was performed using computational resources at both Freie Universität Berlin and the Zuse Institut Berlin. Batch order was fixed to be the same every time the training was restarted/extended. Fig. S4 shows the loss over the validation set of molecules as a function of the training epoch. Training took about 9 days on 16 NVIDIA A100 GPUs.

| | |
|---|---|
| Interaction Blocks | 4 |
| Embedding Feature Size | 128 |
| Lower Cutoff | 0 |
| Upper Cutoff | 15 $\AA$ |
| Distance Expansion Basis | PhysNet [22] |
| Number of Basis Functions | 64 |
| Number of Filters | 128 |
| Output Network | MLP, 2 layers, [128,64] features |
| Output Prediction | Scalar energy, Delta forces |

**Table S6**: Neural network hyperparameters

| | |
|---|---|
| Optimizer | Adam |
| Base Learning Rate | 0.0001 |
| Batch Size | 80 molecules |
| Number of Epochs | 400 |

**Table S7**: Neural network training hyperparameters

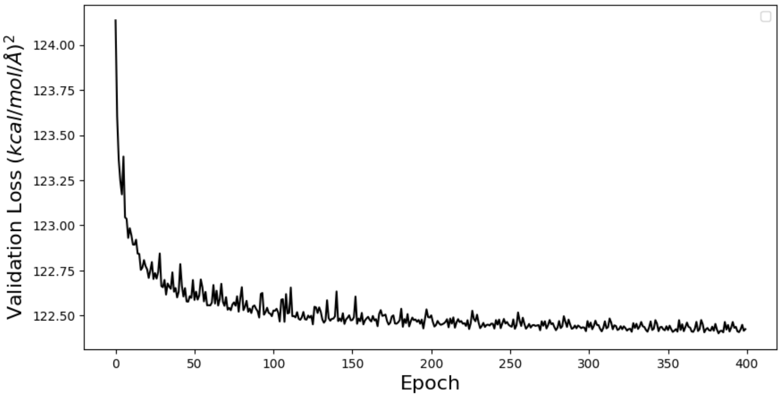


**Fig. S4**: Validation loss for the transferable model as a function of the training epoch number. Note that the validation set contains systems of many different sizes, and as such the absolute loss is not as meaningful. The unoptimizable portion of the force matching loss function is a function of an (unoptimizable) CG mapping operator, a point demonstrated in previous studies [16, 21, 24, 25].

# S4 CG Simulations

## S4.1 Langevin Simulations

Following Husic, Charron, Lemm, et al [24], we conducted Langevin simulations using the following BAOA(F)B integration scheme:

1. $F = -\nabla U(x_t)$

2. $v_{t+1} = v_t + dt\frac{F}{m}$
3. $x_{t+1/2} = x_t + v_t\frac{dt}{2}$
4. $v_{t+1} = v_{t+1/2}\eta_v + dW_t\eta_n$
5. $x_{t+1} = x_{t+1/2}v\frac{dt}{2}$

where $v$ is the instantaneous velocity, $dt$ is the integration timestep, $\eta_v$ and $\eta_n$ are velocity and noise scales respectively, and $dW$ is a stochastic Wiener process. Table S8 contains the specific parameters used in all CGSchNet Langevin simulations. Multiple independent simulations were run on a single GPU in parallel for efficient sampling. The number of trajectories for each protein was chosen as the maximum number of trajectories that could fit on the GPU. For CLN, 50 folded and 50 unfolded configurations were used as starting configurations. For Trpcage, 35 and 35. For BBA, 25 and 25. For Villin, 5 and 5. For A3D, 5 from the folded state. For Homeodomain, 10 from the folded state. For the folding trajectories shown in Fig. 3 of the main text, 5 unfolded starting configurations were also used for Homeodomain and Alpha 3D. For the bigger proteins shown in Fig. 4 of the main text (S6, SH3 and CI2), 5 trajectories were started from the crystal structure and for the IDP (3ZBE) 5 trajectories were started from conformations in the available NMR ensemble.

| | |
|---|---|
| Integrator | Langevin |
| Friction | 1 $ps^{-1}$ |
| Timestep | 4 fs |
| Temperature | 300K |
| Number of steps | (at least) $10^6$ |
| Masses | Atomic |

**Table S8**: CG Langevin simulation parameters

For the four smaller proteins (2RVD, 2JOF, 1FME, and 1YRF), the Langevin simulations were run for $10^6$ steps at first, and convergence of the free energy was checked over time. If necessary, several more millions of MD steps were run until the landscape is converged. The initial 100,000 steps were always discarded for analysis to minimize the impact of the starting structure choices. For the larger proteins, for which we aimed to investigate stability and fluctuations near the native state, simulations were run for at least $10^6$ MD steps (also throwing away the first 100,000 MD steps).

## S4.2 UNRES Simulations

UNRES simulations of extrapolation targets were carried out using the UNRES web server [26, 27]. For each protein, several independent trajectories were run for 10M MD steps each, using all of the default server settings and the latest version of the UNRES force field ("NEWCT-9P" [28]). For three of the four smaller proteins (2RVD, 2JOF, 1FME), 10 trajectories were started from the folded and 10 trajectories were started from the unfolded state. For every other target, 10 independent trajectories were started from the PDB crystal structure. No secondary structure, NMR, or SAXS restraints were used.

## S4.3 AWSEM Simulations

AWSEM simulations were run using the AWSEM-MD code [29]. The simulation parameters used for these simulations are summarized in Table S9. The total simulation time was set to a higher value to ensure correct sampling of the equilibrium NVT ensemble.

| | |
|---|---|
| Integrator | Velocity-Verlet |
| Thermostat | Nose-Hoover |
| Number of Simulations | 10 |
| Damping | 100 fs |
| Timestep | 4 fs |
| Temperature | 300 K |
| Number of steps | 10M |

**Table S9**: AWSEM-MD simulation parameters

The Hamiltonian that was used for these simulations is the one as described in [29]:

$$V_{total} = V_{backbone} + V_{contact} + V_{burial} + V_{HB} + V_{FM} \tag{8}$$

To ensure comparability with our approach and assess the transferability of AWSEM to unseen proteins, only the homologs excluded database was used for the fragment memory term ($V_{FM}$), leaving roughly only sequences in the database that have less than 20% sequence similarity to the target protein. Secondary structure bias was used, but the secondary structure prediction was made using only knowledge of the primary sequence of the target protein to remain comparable with our approach. Secondary structure prediction was made using the JPred server [30] (https://www.compbio.dundee.ac.uk/jpred/, last checked on October 27th, 2023) turning off the option to use a full structure from the PDB if existing.

## S4.4 Parallel-tempering simulations

Following [25], parallel tempering (PT) simulations were performed in order to enhance the sampling. These simulations used the same integrator and integration settings as the Langevin simulations described above. The thermostat temperatures for different replicas range from below to above the target temperature (300K) and were selected as a geometrical progression with the possible exception of the target temperature, which was always included. For all simulations, an exchange between adjacent-temperature replicas is attempted every 2000 simulation steps. The number of replicas was adjusted in order that the acceptance ratio of attempted exchanges between replicas with adjacent temperatures lies around 20% [31]. The number of replicas and temperature range specific to each simulated protein are reported in Table S10.

The free energy surfaces were obtained by reweighting all the simulations to the target temperature through the Weighted Histogram Analysis Method (WHAM) procedure [32] as implemented in PyEmma [33]. The construction of the histogram

required for the reweight was done using k-means clustering in the $Q$-RMSD space with 500 cluster centers.

For 2RVD, 2JOF, 1FME, and 1YRF, the simulations were run for at least 2M MD steps and extended as needed to achieve convergence in the landscape. For the other proteins, the PT simulations were run for at least 2M steps. The analysis was performed after throwing away the first 100,000 steps for all proteins, except 1FME, where the first 900,000 steps were discarded (due to slower system convergence in that case).

| Protein | Temperature range (K) | # replicas | # independent simulations |
|---|---|---|---|
| CLN025 (2RVD) | 200-393.4 | 4 | 50 |
| Trpcage (2JOF) | 200-393.4 | 6 | 24 |
| BBA (1FME) | 200-393.4 | 6 | 18 |
| Villin (1YRF) | 200-406.8 | 8 | 4 |
| Homeodomain (1ENH) | 200-393.5 | 11 | 2 |
| Alpha 3D (2A3D) | 200-393.5 | 11 | 1 |
| S6 (1RIS) | 200-393.5 | 11 | 1 |
| SH3 (2NUZ) | 200-393.5 | 11 | 2 |
| CI2 (2CI2) | 200-393.5 | 11 | 2 |

**Table S10**: Parallel tempering parameters. Independent PT simulations were performed simultaneously to fully exploit the GPU capacity thus reducing the time spent on accumulating sufficient samples.

# S5 Single Protein Test at the Transferable Resolution

In order to rule out potentially poor prior modeling choices at the 5-CG-atom-per-residue resolution, a single-protein (non-transferable) model of CLN025 (2RVD) was trained using the same hyperparameters and training routine as the transferable model and subsequently simulated to see if it could reproduce the free energy landscape of the reference dataset. For the reference dataset, we chose to use the CLN025 dataset (CHARMM22*, 350K) used in previous works [16, 24, 34] and applied the same basic, constraint-aware force mapping strategy as in the transferable dataset. The same set of priors were fit directly to this dataset. The resulting free energy surface (plotted in the same dominant TICA components in the aforementioned studies) obtained from the model aligns very well with the reference as shown in Fig. S5, thereby providing evidence that our prior strategy is at least reasonable for a delta-learning force approach. Additionally, it suggests that the network hyperparameters are expressive enough to model the multibody interactions of the CG PMF (at least for a single protein).

# S6 Prior-only Simulations

It is important to understand how the CGSchNet model is able to learn corrections to the underlying prior model. To this end, we conducted direct MD CG simulations

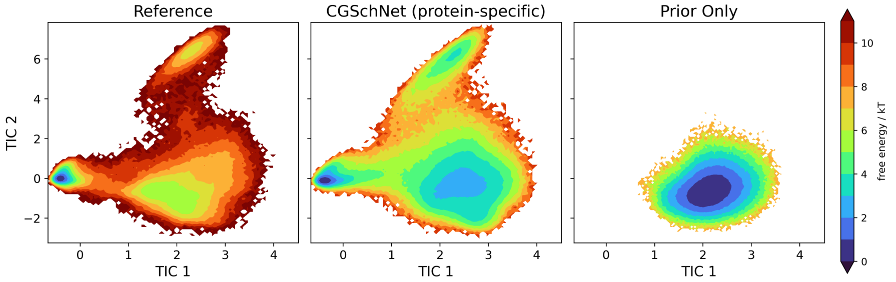


**Fig. S5**: Performance of a single protein model of CLN025 at the transferable resolution quantified by the free energy surface in the space of the first two components of TICA analysis. Left) Reference. Middle) Single-protein CGSchNet. Right) Simulation of prior force field only.

of all proteins for which free energy surfaces are shown in the main text, by using only the prior energy model, thus with no learned parameters; these simulations are shown in Fig. S6. As expected, in the prior-only simulations all proteins unfold and remain unfolded throughout the simulation. Interestingly, while similar results are obtained as with the trained CG model and the reference atomistic simulations for the two 8-residue peptides, the 71-residue intrinsically disordered peptide explores a rather different configurational landscape with respect to CGSchNet when simulated with only the prior energy model. It is thus clear that the simulation results obtained by our trained CG model arise from the ability of the network to learn the necessary multi-bodied interactions and corrections to the underlying prior model.

# S7 Analysis Details

## S7.1 Calculation of Fraction of Native Contacts, $Q$

A common reaction coordinate for protein folding is the fraction of native contacts, $Q$, which characterizes the degree to which a given protein structure is similar to a known native structure. For a protein system with a set of native contacts distances, $\{r_0\}$, defined between a determined set of atom pairs, the value $Q$ of a conformation with distances of the same set of atom pairs $\{r\}$ is defined as:

$$Q(\{r\},\{r_0\}) = \frac{1}{\{r_0\}} \sum_{i}^{|\{r_0\}|} \frac{1}{1+\exp(\beta(r_i - \lambda r_{i,0})} \tag{9}$$

where the sum extends over all contacting pairs. $\beta$ and $\lambda$ control the contact membership smoothing and contact fluctuation allowance, respectively. This measure has been investigated and tuned for analysis of fast-folding proteins at the atomistic resolution [36].

In order to use this reaction coordinate for CG systems the following approach is taken. First, contacting residues (considered for those at least 3 residues apart in

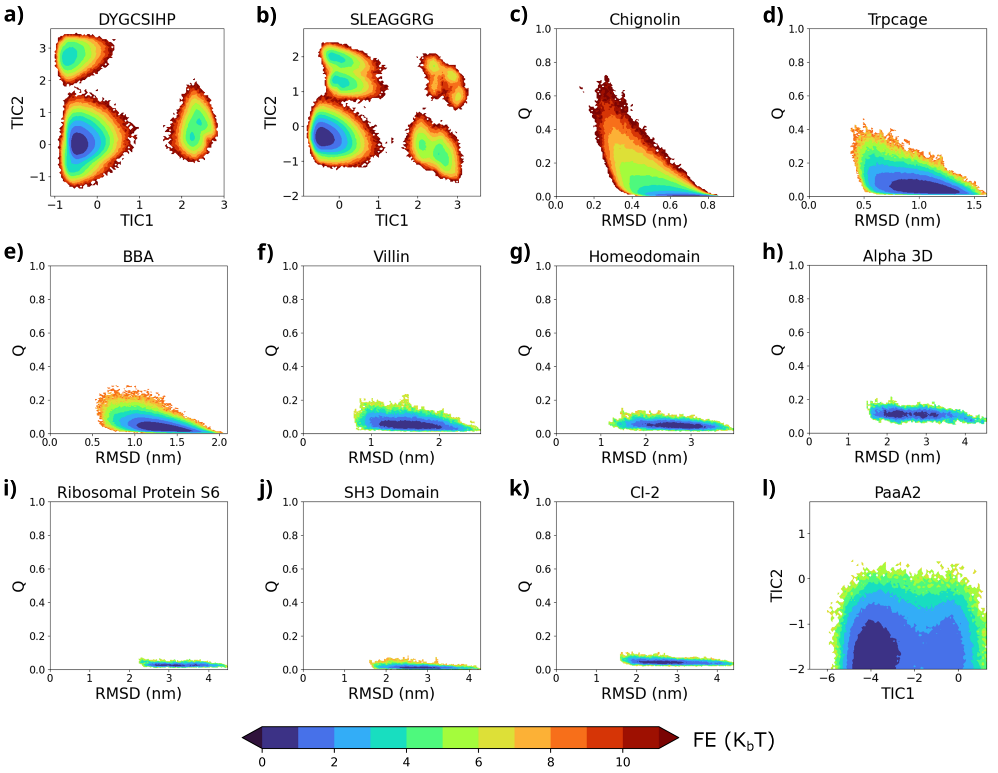


**Fig. S6**: Simulations of all proteins discussed in the main text performed only with a prior energy model, i.e. with no neural network. These proteins consist of a) 8-residue peptide DYGCSIHP, b) 8-residue peptide SLEAGGRG, c) CLN025 (2RVD), d) Trpcage (2JOF), e) BBA (1FME), f) Villin (1YRF), g) Homeodomain (1ENH), h) Alpha3D (2A3D), i) Ribosomal protein S6 (1RIS), j) SH3 domain (2NUZ), k) CI2 (2CI2), and l) antitoxin peptide PaaA2 (3ZBE). All free energy landscapes are shown as a function of RMSD and Q with the exception of the two 8-peptides and PaaA2, where these coordinates cannot be easily defined (no unique folded state). Instead, the landscape is shown as a function of the first two TICA coordinates [35].

sequence) of a native state structure are defined if any two heavy atoms from either residue are within 4.5 $\mathring{A}$ of each other. Rather than recording these distances directly as elements of the set $\{r_0\}$, the distances of the corresponding carbon alpha atoms of the contacting residues are recorded instead. After a set of carbon alpha native contacts is identified, eq. 9 can be used at the carbon alpha resolution, which is applicable to any CG model with a resolution that retains or has knowledge of the carbon alpha atom positions.

Additionally, $\lambda$ and $\beta$ must be adjusted away from their atomistically tuned values of 1.8 and 50 $nm^{-1}$ respectively. Due to the higher positional rigidity of backbone carbon alpha atoms compared to sidechain atoms normally used to determine contacts, $\lambda$ must be reduced so that larger backbone rearrangements are not counted in the same

contact [36]. To this end, we set $\lambda = 1.5$, following the investigations of backbone-resolution CG Go-MARTINI protein models [37]. Additionally, we set $\beta = 10$ nm$^{-1}$ to prevent systematic artifacts/ringing in the free energy at integral fractions of residues. This set of $\lambda$ and $\beta$ allows for interpretable and smooth free energy surfaces that can be employed for CG analysis of any protein in this study, all of which clearly separate native/native-like configurations from unfolded configurations (i.e., $Q \approx 1$ for configurations close to the native structure).

## S7.2 Calculation of the Root Mean Square Fluctuations

For the computation of the $C_\alpha$ Root Mean Square Fluctuations (RMSF) inside the folded state shown in Fig. 3, one trajectory starting from the folded state was chosen for each protein. A window of frames maintaining the folded state for at least 1 million MD steps was chosen to compute the $C_\alpha$ RMSF. The chosen trajectories and windows for both Homeodomain and alpha3D are shown in Fig. S7.

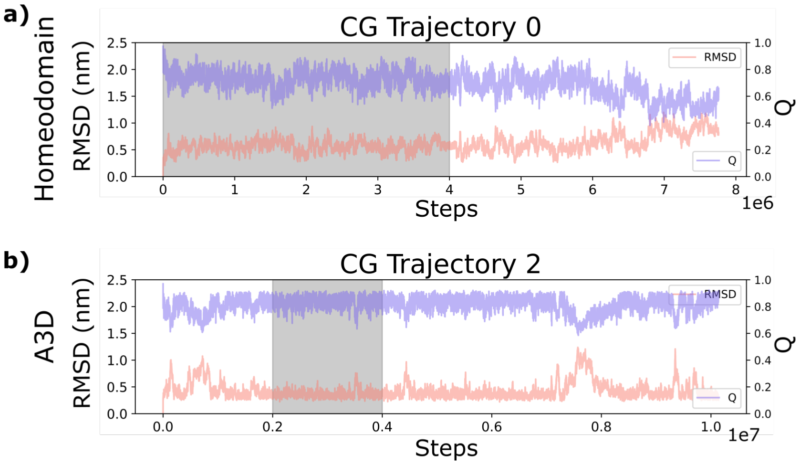


**Fig. S7**: Trajectory windows used for the computation of the $C_\alpha$ Root Mean Square Fluctuations for Homeodomain (1ENH) and alpha3D (2A3D).

## S7.3 GDT-TS Calculations

The Global Distance Test (GDT) [38] was introduced as a more refined alternative to RMSD measurements for protein structure comparisons, being less sensitive to disordered regions. For a chosen distance cutoff, $r_{GDT}$, the GDT consists of finding the largest set of (potentially non-contiguous) matching protein residues between a query and a target structure whose corresponding carbon alpha pair distances differ by no more than $r_{GDT}$. The GDT algorithm converges to a static set of maximally superimposable residues, and the output is given as a percentage of the total number of residues in the target structure. The GDT-TS ("Global Distance Test Total Score") is reported as the average percentage of maximally superimposeable residues from

running the GDT algorithm for multiple $r_{GDT}$ choices. The CASP3 structure prediction competition officially adopted the GDT-TS as a measure of how accurately a model-generated query structure matched a target structure for $r_{GDT} = 1, 2, 4, 8$ Å cutoffs [39]. As the GDT-TS only requires knowledge of query and target structures' carbon alpha atom positions, it can be used without modification for any CG model that retains knowledge of these atoms. In all GDT-TS measurements for any CG model in this manuscript, the default cutoff series ($r_{GDT} = 1, 2, 4, 8$ Å) is used. All GDT-TS computations were done using the Zhang lab C++ standalone implementation of the TM-score program [40].

## S7.4 Computation of the structural metrics and ensembles of structures

For each protein and each model, a free energy surface was plotted in Q vs. RMSD space (or as a function of the two first TICA components [35] in the case of Fig. 5) excluding the first 10% of the simulation for AWSEM and UNRES simulations and the first 100,000 MD steps for the CGSchNet simulations. This free energy surface was clustered using k-means clustering and the number of clusters shown in table S3 for Fig. 5 or 100 cluster centers for the computation of the structural metrics. The cluster best representing the interesting basins was chosen by visual inspection and 10 structures were pulled from there. The structures pulled from the most folded-like metastable basins in RMSD vs. Q space (lowest RMSD/highest Q) were used to compute the GDT-TS score. The positions of the most folded-like cluster centers on the free energy surface for each protein and each force field can be checked in Fig. S10. The probability density of the fraction of native contacts (Q) was computed for the same part of the simulations, and a smoothed version was plotted using a Savitzky-Golay filter of order 10 (5 for 1ENH) [19, 41]. The order was chosen to give consistent results on all simulations of the same protein, minimizing the smoothing artifacts and making sure that the remaining artifacts did not impact the detection of the right peak. The relative maxima of the smoothed Q probability density were computed using scipy and the highest Q value corresponding to a relative maximum in probability density was plotted to be the largest metastable Q. Smoothed Q probability densities and largest metastable Q for each protein and each model can be found in Fig. S10, while the structures pulled for GDT-TS are aligned with the reference and visualized in Fig. S11.

## S7.5 Comparison with DESRES simulations

It is interesting to measure the structural metrics also on the results of atomistic simulations from D.E. Shaw research group [14] (called DESRES simulations hereafter). In Fig. S8 we show that even for these atomistic simulations the GDT-TS score is not always close to 1. In particular, in the case of Homeodomain, the folded-like metastable state is at a Q-value around 0.6, as in our CG model. Note that the DESRES simulations were carried out with a different force field and at a different temperature than the one used for the generation of the training data. Also note two differences in

sequence between the DESRES simulations and the other CG force fields: the Homeodomain sequence used in the DESRES simulations corresponds to PDB code 2P6J, which is different from the 1ENH sequence used for this study. In the 1YRF sequence, NLE was mutated to LEU in our study to account for the lack of embedding for NLE in our training data.

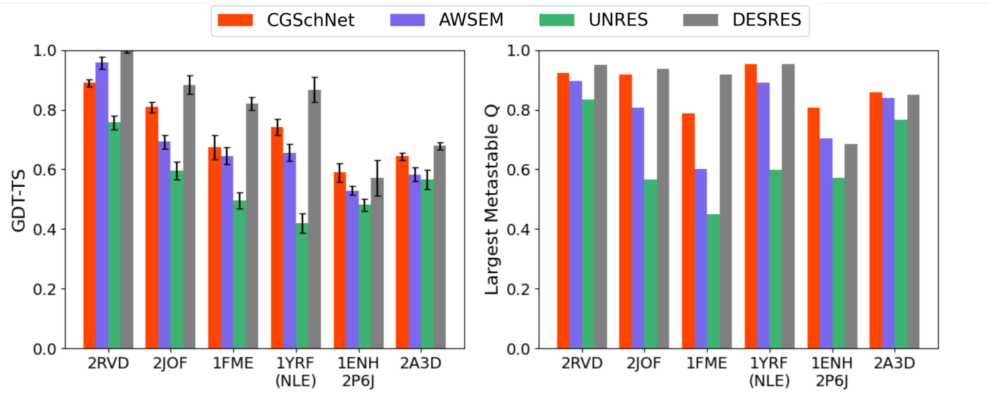


**Fig. S8**: Computation of the structural metrics on structures pulled from the most folded-like basins of the free energy in Q vs. RMSD space for the three CG force-fields shown in Fig. 5 of the main text as well as for the DESRES simulations.

## S7.6 Comparison between Langevin and PT simulations

In order to demonstrate the stability of our model under various simulation setups and techniques, we present a comparison of the free energy landscape obtained through Langevin and PT simulations in Fig. S9. As in the main text, the free energy is reported as a function of the fraction of native contact and carbon alpha RMSD to the native state.

## S7.7 Speed-up calculation

The relative speed-up between the AA and the CG model was estimated from our simulations. The speed-up factor can be decomposed into two parts: (1) The decorrelation time, or slowest relaxation time, $\tau$ is the value of the implied timescale of the slowest process according to an MSM built over the trajectories of the simulation. For the systems here the slowest process is typically the folding/unfolding transition; (2) The "speed of simulation" $v$ measures the computational cost of one simulation step on the same reference GPU. We can quantify the speed-up with the following formula

$$s = \frac{\tau^{(AA)}}{\tau^{(CG)}} \frac{v^{(CG)}}{v^{(AA)}} \tag{10}$$

where $AA$ and $CG$ stand for all-atom and coarse-grained, respectively.

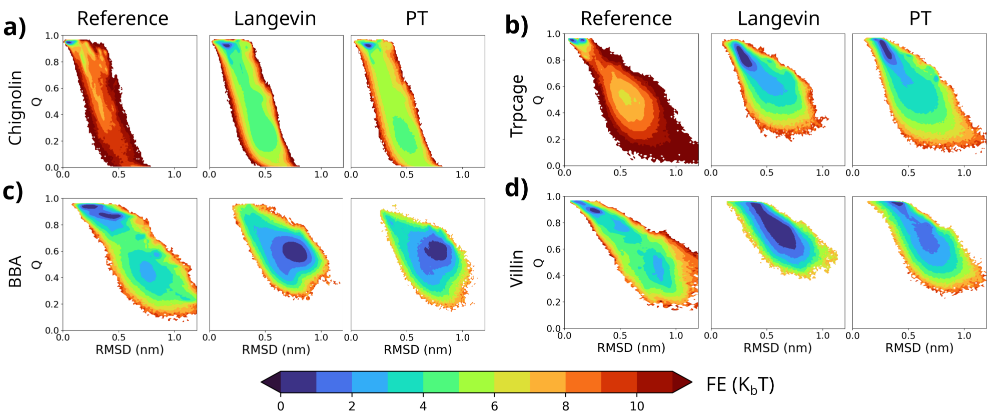


**Fig. S9**: Comparison of PT and Langevin simulations for the four small proteins shown in the main text: a) CLN025 (2RVD), b) Trpcage (2JOF), c) BBA (1FME), and d) Villin (1YRF).

The CG simulation times were estimated from Langevin simulations with the temperature set to the same as the corresponding AA simulations. Parallel tempering simulations are not considered here because the transitions are partially due to temperature swaps and are therefore not used to infer the physical transition time. The results of the speed-up calculation can be found in Table S11.

| Protein | $\tau^{(AA)}$ ($TS_{AA}$) | $\tau^{(CG)}$ ($TS_{CG}$) | $v^{(AA)}$ ($TS_{AA}$/s) | $v^{(CG)}$ ($TS_{CG}$/s) | Speed up |
|---|---|---|---|---|---|
| CLN025 | $2.27\times10^8$ | $1.10\times10^5$ | $4.08\ \times10^3$ | 57.1 | 29.1 |
| Trpcage | $1.71\times10^9$ | $6.44\times10^4$ | $2.49\ \times10^3$ | 53.2 | 565.7 |
| BBA | $9.73\times10^8$ | $1.70\times10^5$ | $2.49\ \times10^3$ | 55.6 | 127.9 |
| Villin | $1.48\times10^{10}$ | $1.28\times10^6$ | $4.05\ \times10^3$ | 52.4 | 151.9 |

**Table S11**: Speed-up calculation. Times for the AA simulations are presented in AA timestep (TS) = 2 fs. The simulation speeds $v$ were measured on a single Nvidia A5000 GPU

The reported CG simulation speed $v^{(CG)}$ is not affected by the molecular size, since the wall time spent for each time step is dominated by the hardware communication overhead. In practice, multiple simulations can be executed in parallel to saturate the computation capacity of a GPU by amortizing the overhead of hardware communication, which usually brings 5 20x throughput. It is also worth noting that this speed-up is achieved even though the MD simulations of our CG model were performed with our in-house code, which is not optimized for performance. The MD simulations for the reference atomistic model were performed with OpenMM, which is highly optimized. In general, MD simulations with neural network potentials are still very expensive compared to classical force fields.

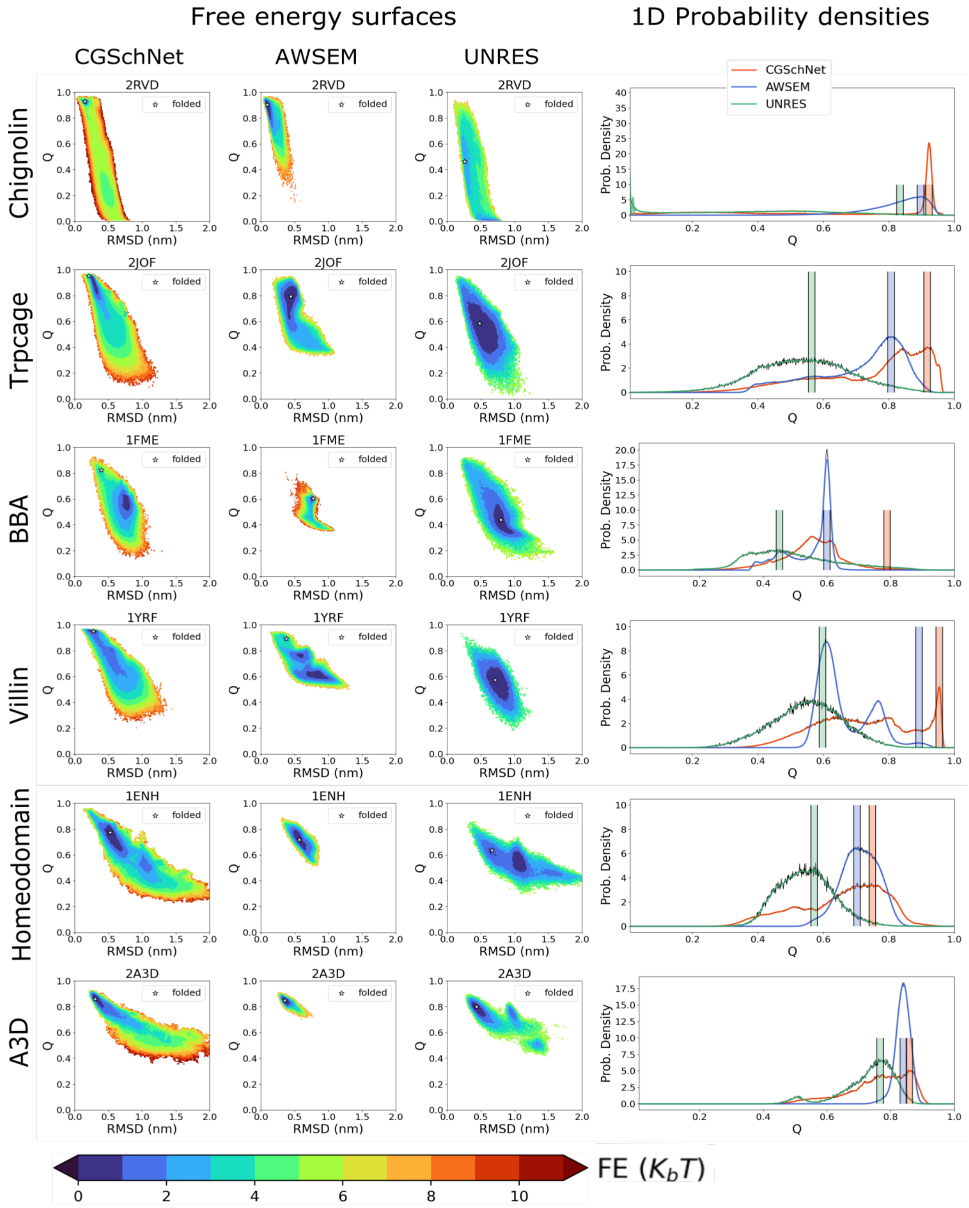


**Fig. S10**: Details on the computation of the structural metrics shown in Figure 5 of the main text. For each protein and each CG force field, the free energy surface in Q vs. RMSD space and the most folded-like cluster center, from which structures for the computation of the GDT-TS score were extracted, are plotted. On the right, the smoothed probability densities over Q are plotted, as well as the largest metastable Q detected.

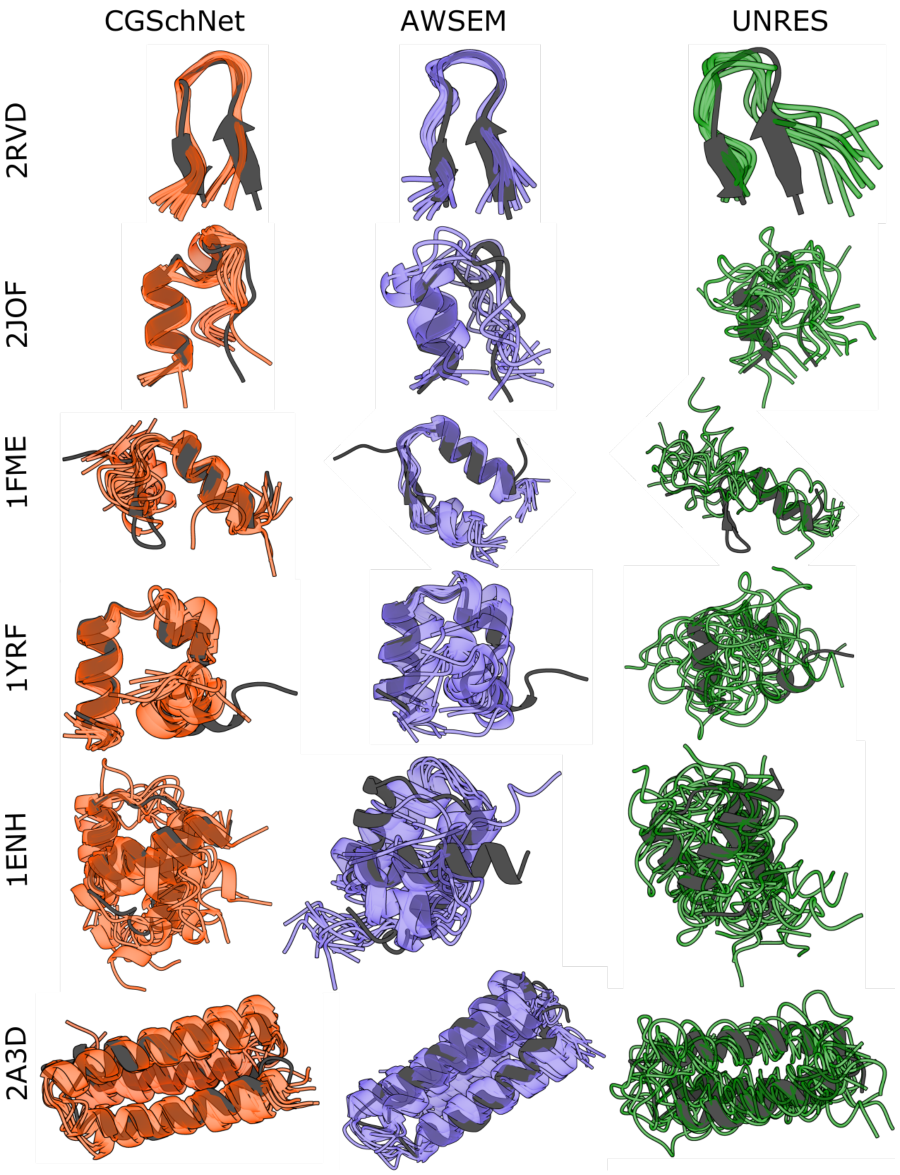


**Fig. S11**: Ensemble of structures pulled for the computation of the GDT-TS score for each protein and each CG force-field. Subfigures generated using UCSF ChimeraX [13].

# References


[1] Wang, G., Dunbrack, R.L.: Pisces: a protein sequence culling server. Bioinformatics **19**(12), 1589–1591 (2003)

[2] Zimmerman, J.M., Eliezer, N., Simha, R.: The characterization of amino acid sequences in proteins by statistical methods. J. Theor. Biol. **21**(2), 170–201 (1968)

[3] Lindorff-Larsen, K., Piana, S., Palmo, K., Maragakis, P., Klepeis, J.L., Dror, R.O., Shaw, D.E.: Improved side-chain torsion potentials for the amber ff99sb protein force field. Proteins **78**(8), 1950–1958 (2010)

[4] Jorgensen, W.L., Chandrasekhar, J., Madura, J.D., Impey, R.W., Klein, M.L.: Comparison of simple potential functions for simulating liquid water. J. Chem. Phys. **79**(2), 926–935 (1983)

[5] Schrödinger, L.: The PyMOL Molecular Graphics System, Version 1.8 (2015)

[6] Harvey, M.J., Giupponi, G., Fabritiis, G.D.: Acemd: Accelerating biomolecular dynamics in the microsecond time scale. J. Chem. Theory Comput. **5**(6), 1632–1639 (2009)

[7] Doerr, S., De Fabritiis, G.: On-the-fly learning and sampling of ligand binding by high-throughput molecular simulations. J. Chem. Theory Comput. **10**(5), 2064–2069 (2014)

[8] Eastman, P., Swails, J., Chodera, J.D., McGibbon, R.T., Zhao, Y., Beauchamp, K.A., Wang, L.-P., Simmonett, A.C., Harrigan, M.P., Stern, C.D., Wiewiora, R.P., Brooks, B.R., Pande, V.S.: Openmm 7: Rapid development of high performance algorithms for molecular dynamics. PLOS Comput. Biol. **13**(7), 1005659 (2017)

[9] Sillitoe, I., Lewis, T.E., Cuff, A., Das, S., Ashford, P., Dawson, N.L., Furnham, N., Laskowski, R.A., Lee, D., Lees, J.G., Lehtinen, S., Studer, R.A., Thornton, J., Orengo, C.A.: Cath: comprehensive structural and functional annotations for genome sequences. Nucleic Acids Res. **43**(D1), 376–381 (2015)

[10] Kabsch, W., Sander, C.: Dictionary of protein secondary structure: pattern recognition of hydrogen-bonded and geometrical features. Biopolymers **22**(12), 2577–2637 (1983)

[11] McGibbon, R.T., Beauchamp, K.A., Harrigan, M.P., Klein, C., Swails, J.M., Hernández, C.X., Schwantes, C.R., Wang, L.-P., Lane, T.J., Pande, V.S.: Mdtraj: A modern open library for the analysis of molecular dynamics trajectories. Biophys. J. **109**(8), 1528–1532 (2015)

[12] Abraham, M.J., Murtola, T., Schulz, R., Páll, S., Smith, J.C., Hess, B., Lindahl, E.: Gromacs: High performance molecular simulations through multi-level

parallelism from laptops to supercomputers. SoftwareX **1**, 19–25 (2015)

[13] Goddard, T.D., Huang, C.C., Meng, E.C., Pettersen, E.F., Couch, G.S., Morris, J.H., Ferrin, T.E.: Ucsf chimerax: Meeting modern challenges in visualization and analysis. Protein Sci. **27**(1), 14–25 (2018)

[14] Lindorff-Larsen, K., Piana, S., Dror, R.O., Shaw, D.E.: How fast-folding proteins fold. Science **334**(6055), 517–520 (2011)

[15] Husic, B.E., Pande, V.S.: Markov state models: From an art to a science. J. Am. Chem. Soc. **140**, 2386–2396 (2018)

[16] Majewski, M., Pérez, A., Thölke, P., Doerr, S., Charron, N.E., Giorgino, T., Husic, B.E., Clementi, C., Noé, F., De Fabritiis, G.: Machine learning coarse-grained potentials of protein thermodynamics. Nat. Commun. **14**(1), 5739 (2023)

[17] Hoffmann, M., Scherer, M., Hempel, T., Mardt, A., Silva, B., Husic, B.E., Klus, S., Wu, H., Kutz, N., Brunton, S.L., Noé, F.: Deeptime: a python library for machine learning dynamical models from time series data. Mach. Learn.: Sci. Technol. **3**, 015009 (2022)

[18] Cock, P.J., Antao, T., Chang, J.T., Chapman, B.A., Cox, C.J., Dalke, A., Friedberg, I., Hamelryck, T., Kauff, F., Wilczynski, B., *et al.*: Biopython: freely available python tools for computational molecular biology and bioinformatics. Bioinformatics **25**(11), 1422–1423 (2009)

[19] Virtanen, P., Gommers, R., Oliphant, T.E., Haberland, M., Reddy, T., Cournapeau, D., Burovski, E., Peterson, P., Weckesser, W., Bright, J., van der Walt, S.J., Brett, M., Wilson, J., Millman, K.J., Mayorov, N., Nelson, A.R.J., Jones, E., Kern, R., Larson, E., Carey, C.J., Polat, İ., Feng, Y., Moore, E.W., VanderPlas, J., Laxalde, D., Perktold, J., Cimrman, R., Henriksen, I., Quintero, E.A., Harris, C.R., Archibald, A.M., Ribeiro, A.H., Pedregosa, F., van Mulbregt, P., SciPy 1.0 Contributors: SciPy 1.0: Fundamental Algorithms for Scientific Computing in Python. Nat. Methods **17**, 261–272 (2020)

[20] Schütt, K.T., Kessel, P., Gastegger, M., Nicoli, K.A., Tkatchenko, A., Müller, K.-R.: Schnetpack: A deep learning toolbox for atomistic systems. J. Chem. Theory Comput. **15**(1), 448–455 (2019)

[21] Wang, J., Olsson, S., Wehmeyer, C., Pérez, A., Charron, N.E., Fabritiis, G., Noé, F., Clementi, C.: Machine learning of coarse-grained molecular dynamics force fields. ACS Cent. Sci. **5**(5), 755–767 (2019)

[22] Unke, O.T., Meuwly, M.: Physnet: A neural network for predicting energies, forces, dipole moments, and partial charges. J. Chem. Theory Comput. **15**(6), 3678–3693 (2019)

[23] Falcon, W., The PyTorch Lightning team: PyTorch Lightning. https://github.com/Lightning-AI/lightning

[24] Husic, B.E., Charron, N.E., Lemm, D., Wang, J., Pérez, A., Krämer, A., Chen, Y., Olsson, S., Fabritiis, G., Noé, F., Clementi, C.: Coarse graining molecular dynamics with graph neural networks. J. Chem. Phys. **153**(19), 194101 (2020)

[25] Chen, Y., Krämer, A., Charron, N.E., Husic, B.E., Clementi, C., Noé, F.: Machine learning implicit solvation for molecular dynamics. J. Chem. Phys. **155**(8), 084101 (2021)

[26] Czaplewski, C., Karczynska, A., Sieradzan, A.K., Liwo, A.: Unres server for physics-based coarse-grained simulations and prediction of protein structure, dynamics and thermodynamics. Nucleic Acids Res. **46**(W1), 304–309 (2018)

[27] Slusarz, R., Lubecka, E.A., Czaplewski, C., Liwo, A.: Improvements and new functionalities of unres server for coarse-grained modeling of protein structure, dynamics, and interactions. Front. Mol. Biosci **9** (2022)

[28] Liwo, A., Sieradzan, A.K., Lipska, A.G., Czaplewski, C., Joung, I., Zmudzinska, W., Halabis, A., Oldziej, S.: A general method for the derivation of the functional forms of the effective energy terms in coarse-grained energy functions of polymers. iii. determination of scale-consistent backbone-local and correlation potentials in the unres force field and force-field calibration and validation. J. Chem. Phys. **150**(15), 155104 (2019)

[29] Davtyan, A., Schafer, N.P., Zheng, W., Clementi, C., Wolynes, P.G., Papoian, G.A.: AWSEM-MD: protein structure prediction using coarse-grained physical potentials and bioinformatically based local structure biasing. J. Phys. Chem. B **116**(29), 8494–8503 (2012)

[30] Drozdetskiy, A., Cole, C., Procter, J., Barton, G.J.: JPred4: a protein secondary structure prediction server. Nucleic Acids Res. **43**(W1), 389–394 (2015)

[31] Rathore, N., Chopra, M., Pablo, J.J.: Optimal allocation of replicas in parallel tempering simulations. J. Chem. Phys. **122**(2) (2005)

[32] Andrec, M.: The weighted histogram analysis method (WHAM). Citeseer (2010)

[33] Scherer, M.K., Trendelkamp-Schroer, B., Paul, F., Pérez-Hernández, G., Hoffmann, M., Plattner, N., Wehmeyer, C., Prinz, J.-H., Noé, F.: PyEMMA 2: A Software Package for Estimation, Validation, and Analysis of Markov Models. J. Chem. Theory Comput. **11**, 5525–5542 (2015)

[34] Krämer, A., Durumeric, A.E.P., Charron, N.E., Chen, Y., Clementi, C., Noé, F.: Statistically optimal force aggregation for coarse-graining molecular dynamics. J. Phys. Chem. Lett. **14**(17), 3970–3979 (2023)

[35] Pérez-Hernández, G., Paul, F., Giorgino, T., De Fabritiis, G., Noé, F.: Identification of slow molecular order parameters for markov model construction. J. Chem. Phys. **139**(1), 015102 (2013)

[36] Best, R.B., Hummer, G., Eaton, W.A.: Native contacts determine protein folding mechanisms in atomistic simulations. Proc. Natl. Acad. Sci. U.S.A. **110**(44), 17874–17879 (2013)

[37] Poma, A.B., Cieplak, M., Theodorakis, P.E.: Combining the martini and structure-based coarse-grained approaches for the molecular dynamics studies of conformational transitions in proteins. J. Chem. Theory Comput. **13**(3), 1366–1374 (2017)

[38] Zemla, A.: Lga: a method for finding 3d similarities in protein structures. Nucleic Acids Res. **31**(13), 3370–3374 (2003)

[39] Zemla, A., Venclovas, C., Moult, J., Fidelis, K.: Processing and analysis of casp3 protein structure predictions. Proteins **37**(S3), 22–29 (1999)

[40] Zhang, Y., Skolnick, J.: Scoring function for automated assessment of protein structure template quality. Proteins **57**(4), 702–710 (2004) https://doi.org/10.1002/prot.20264

[41] Savitzky, A., Golay, M.J.E.: Smoothing and differentiation of data by simplified least squares procedures. Anal. Chem. **36**(8), 1627–1639
